# Supplementary material for: Slot-Level Robotic Placement via Visual Imitation from Single Human Video
Source: arXiv:2504.01959 source file (2025-04-02)
Supplement: Supplementary file 1 [file supp_test.tex]

% \begin{tabular}{|c|c|}
% \hline
% \textbf{Text} & \textbf{Image} \\ \hline
% \makecell[t]{First line of text \\ Second line of text} & 
% \makecell[t]{\includegraphics[width=2cm]{example-image}} \\ \hline
% \makecell[t]{Another text entry} & 
% \makecell[t]{\includegraphics[width=2cm]{example-image}} \\ \hline
% \end{tabular}

% \begin{tabular}{c|l}
% \textbf{Verb}   & \textbf{Example}   \\ \hline
% ``goes-to''     & \includegraphics[scale=0.1,valign=c]{example-image-a} \\[1em] \hline
% ``walks-to''    & \includegraphics[scale=0.1,valign=c]{example-image-a}    \\[1em] \hline
% ``says to''     &  \includegraphics[scale=0.1,valign=c]{example-image-a}      \\[1em] \hline
% ``chats to''    &\includegraphics[scale=0.1,valign=c]{example-image-a}
% \end{tabular}
